# Supplementary material for: Klout Topics for Modeling Interests and Expertise of Users Across Social Networks
Source: arXiv:1710.09824 source file (2017-10-26)
Supplement: Supplementary file 1 [file ontology_appendix.tex]

\subsection{Overview of Development}

\subsection{Bootstrapping the Ontology}
The first version of the ontology consisted of 140k nodes from the following sources: 
\begin{enumerate}
\item Keywords extracted from processed tweets
\item (Which academic topic sets? need reference) 
\end{enumerate}

A team of employees was tasked with whittling down the set of topics by removing those that were:
\begin{itemize}
\item too specific to be applied to a significant number of profiles or URLs (``Offices of Dentists (Industry)'', ``Australian Desert Raisin (Ingredient)'')
\item too general or ambiguous to be meaningful (``Minister-President'', ``Comments'', ``Short List'')
\item out of date (``Seattle Supersonics (Basketball)'')
\item containing profanity or adult content (``Tits \& Clits Comix (Comic Books)'')
\end{itemize} 
This approach resulted in a set of ~10,000 v1 topics. Each topic node contained a unique numerical identifier, a human-readable string identifier, an English-language display\_name, and a ``type'' field indicating where it lay within the ontology's tree structure (see below).

The same team was then tasked with verifying parent-child relationships inferred from Freebase's data structure. A stand-alone tool was created for this task, which required (time estimate).  

v1 topics were organized into a three-level tree:
\begin{itemize} 
\item Supertopics: 15 top-level domains, e.g. ``Business'' and ``Entertainment''
\item Subtopics: \~1000 more specific categories, such as ``Accounting'' and ``Music''. Each subtopic is limited to a single parent at the supertopic level.
\item Entities: \~9000 named ``entities'' or more specific topics, such as ``TurboTax'' or ``Lady Gaga''. Each entity may have multiple parents, but at the subtopic level only. (todo: clarify definition of entities here versus in Papyrus)
\end{itemize}

A dedicated ontology specialist was brought on to normalize topic names and handle ongoing curation and maintenance. 
This included normalizing names from the formal, parenthesis-heavy academic labels; adding missing topics too new or simply overlooked in Freebase; and deleting duplicate concepts.

v1 of the ontology had several drawbacks. 
First, the three-level limit caused a pile-up at the bottommost (``entity'') level, where topics that should have had a parent-child relationship were forced into a sibling one instead; for example, v1 contained both \textbf{Sports and Recreation > Baseball > Major League Baseball} and \textbf{Sports and Recreation > Baseball > Boston Red Sox}, where the preferred path would be \textbf{Sports and Recreation > Baseball > Major League Baseball > Boston Red Sox}. 
Similarly, the restriction on the allowed level of a parent topic meant that not all possible paths could be represented; the v1 ontology could support either \textbf{Hobbies > Antiques} or \textbf{Lifestyle > Home Decorating > Antiques}, but not both.

An even more pressing problem from a business perspective was that the v1 ontology could only support a single display\_name, and therefore could not be internationalized without supporting multiple parallel versions. 

\subsection{Ontology Development}
Beginning in 2014, we began developing an improved version of the Klout ontology, incorporating the following changes. 
(More about the characteristics of ontology v2 can be found in section 5, below.)

First, v2 removed restrictions on number and level of parent topics, moving from a topic tree to a directed graph. 
We retained the original set of top-level topics, but now allow multiple parents at any level so long as the resulting path is not recursive. 

Next, we added internationalization as an additional dimension of metadata attached to the topic node; now every node includes multiple display\_names in supported languages. 
From both a technical and curation standpoint, we found this approach preferable to maintaining parallel ontologies by language or region. 
While some topics are certainly rooted in a given region or language and will be less frequently found elsewhere (''Toronto Film Festival'', for example), the parent topics will be unchanged, so there is no need to maintain a separate graph. 
Furthermore, adding internationalization to the existing ontology gave us a ``cold start'' for those languages, from which we can work to incrementally improve topic coverage for non-US-English concepts and domains. 
Each display\_name also comes with a flag to indicate whether the given topic should be shown or hidden for the given language, allowing some pruning of less-regionally-relevant topics on the front end.

All internationalization within the ontology is handled at the language level, not the country or other region. 
For business reasons, we also may enforce the hiding of particular topics within particular regions (for example, ``LGBT'' and similar topics within Saudi Arabia). 
However, because those are business decisions that can vary widely by circumstance and application, we chose not to encode those within the ontology itself.

Finally, v2 adds a pointer to the primary Freebase entity for each topic. 
This provides a richer data set for machine learning or text-processing applications.

\subsection{Lessons Learned and Best Practices}
% TODO: revise as advice for others facing similar problems

While much has been written about formal ontology construction, especially for semantic web applications, less has been said about the practical realities of lightweight ontology construction for an enterprise or commercial user-facing application. 
The following are some of the most important lessons learned during the construction, implementation and maintenance of the Klout topic ontology.

\textbf{Expectation of Curation and Incremental Change}. 
An ontology is a living knowledge artifact; it must be clear throughout the organization that building one requires an ongoing investment in the form of time, tools, and documentation. 
Even when choosing to adopt an externally created ontology, it's crucial to consider when and how to propogate updates, whether they come from the external ontology's original creators, or from inside one's own organization. 

\textbf{Clear Chain of Ownership and Documentation}. 
Because an ontology is a living artifact, it should be clear what teams or persons have the authority to make changes. Those owners should document the principles used to make changes, addressing the ontology's scope, structure, and voice. 
A transparent historical record of changes to the ontology is also recommended.

\textbf{Limiting Assumptions}. 
Encoding too many assumptions into your ontology can be dangerous, especially when it spans multiple domains. 
As we saw above, v1 of the Klout ontology was unsatisfactory in part because it assumed both that the top-level categories were mutually exclusive and that there was no need for a path longer than three nodes. 
Fewer rules to enforce can, paradoxically, lead to a cleaner ontology, as well as saving development and curation time.

\textbf{Inclusivity and Tone}. 
Especially if your ontology will be used to visibly classify persons, it is a matter of business importance to be as inclusive as possible. 
Your ontology will reflect your organization's values in the eyes of many users. 
Strive for both caution and consistency when dealing with ideologically controversial concepts, adult concepts, and so forth.

\textbf{Storage Formats and Tools for Curation}. 
There are a range of approaches to storing and describing ontologies, from OWL and Protege, to XTM topic maps, to simple tables in SQL and similar databases. (TODO: Add references) Because ours is a lightweight ontology with a single relationship type, and to make it easier to integrate our ontology with the rest of the data processing pipeline, we chose the straightforward table method, with some temporary front-end tools spun up when needed. This tradeoff has often required the rules of the ontology to be enforced by curators rather than within the tool, emphasizing the importance of clear documentation and quality assurance (see below).

\subsubsection{Metrics and Quality Assurance}.
Like any feature, an ontology in active use should be monitored for quality issues. 
However, it can be difficult to quantify an ontology's issues apart from those of its application. 
When maintaining the Klout ontology, we consider the following:

\textbf{Coverage, a.k.a. Missing Topics}. 
Misapplied topics application can indicate a gap in the ontology, where a less appropriate or too general topic is being used for lack of a better alternative. 
Topics that are missing because they are new concepts can often be identified through current news and tools like Google Trends.

\textbf{Scope, a.k.a. Unneeded Topics}. 
Topics not being applied in the application are often topics that are unneeded. 
Some of these will be topics that were once relevant but are now obsolete and can be safely ``aged out'' of the ontology. 
This is especially true of constantly evolving areas like consumer electronics, movies and television.

\textbf{Missing and Incorrect Edges}. 
Detecting missing or incorrect edges is one of the most difficult areas of ontology improvement. 
Because the Klout ontology does encode references to Freebase, we can compare our edges to Freebase and to some extent to Wikipedia.

\textbf{Application Metrics and User Feedback}. 
Application-level metrics are undeniably useful, although some investigation is required to determine when the cause lies in the ontology and when it lies in some other part of the application. 
There should be a clear path for user feedback about topic assignments.

\textbf{Validation Against Other Ontologies}. 
Validating against other available ontologies is time-consuming, since it requires aligning the ontologies to be compared, but can be revealing. 
See Section 6.
